# Supplementary material for: Certifiable Reachability Learning Using a New Lipschitz Continuous Value Function
Source: arXiv:2408.07866 source file (2025-02-16)
Supplement: Supplementary file 1 [file appendix.tex]

% {\appendix[Proof of the Zonklar Equations]
% Use $\backslash${\tt{appendix}} if you have a single appendix:
% Do not use $\backslash${\tt{section}} anymore after $\backslash${\tt{appendix}}, only $\backslash${\tt{section*}}.
% If you have multiple appendixes use $\backslash${\tt{appendices}} then use $\backslash${\tt{section}} to start each appendix.
% You must declare a $\backslash${\tt{section}} before using any $\backslash${\tt{subsection}} or using $\backslash${\tt{label}} ($\backslash${\tt{appendices}} by itself
%  starts a section numbered zero.)}

\section*{Appendix}

\begin{proof}[Proof of Theorem~\ref{thm:Bellman}]
We first show that $\Bellmanbackup[\valuepure(x)] = \valuepure(x)$, and then prove that $\Bellmanbackup$ is a contraction mapping.  
%We first show that $\valuepure(x)$ as defined in \eqref{eq:inf_horizon_reach_avoid_problem} satisfies the Bellman backup equation \eqref{eq:bellman_backup}, and then show that the proposed Bellman backup \eqref{eq:bellman_backup} is a contraction mapping.

By definition, we have
\begin{equation*}\small
\begin{aligned}
\valuepure(x_0) =& %\inf_{\phi}\max_{\{u_t\}_{t=0}^\infty} \sup_{t=0,1,\dots} \min\Big\{ \gamma^t r(\xi_{x_0}^{\mathbf{u},\phi(\mathbf{u})}(t)), \\&\min_{\tau=0,\dots,t} \gamma^{\tau} c(\xi_{x_0}^{\mathbf{u},\phi(\mathbf{u})}(\tau)) \Big\}\\
%= & \inf_{\phi} \max_{\{u_t\}_{t=0}^\infty}\max\Big\{\min\{r(x_0),c(x_0)\} , \sup_{t=1,2,\dots}\\&  \min\{\gamma^t r(\xi_{x_0}^{\mathbf{u},\phi(\mathbf{u})}(t)), \min_{\tau=0,\dots,t} \gamma^{\tau} c(\xi_{x_0}^{\mathbf{u},\phi(\mathbf{u})}(\tau))\} \Big\}\\
%= &\max \Big\{ \min\{r(x_0), c(x_0)\}, \inf_{\phi}\max_{\{u_t\}_{t=0}^\infty} \sup_{t=1,2,\dots, } \\&\min\{ \gamma^t r(\xi_{x_0}^{\mathbf{u},\phi(\mathbf{u})}(t)),\min_{\tau=0,\dots, t} \gamma^{\tau}c(\xi_{x_0}^{\mathbf{u},\phi(\mathbf{u})}(\tau)) \}  \Big\}\\
\max\Big\{ \min\{ r(x_0), c(x_0) \},   \max_{\controlpolicy}\min_{\disturbancepolicy} \sup_{t=1,2,\dots} \min \{ \min\{\\&\gamma^t r(x_t), \min_{\tau=1,\dots, t} \gamma^{\tau} c(x_\tau)\}, c(x_0) \}\Big\} .
\end{aligned}
\end{equation*}
% We continue the above derivation as,
%The above inequality can be simplified as
Grouping terms with $t\in\{1,2,\dots\}$ as $\valuepure(x_1)$, we have
\begin{equation*}\small
\begin{aligned}
%=&\max\Big\{ \min\{r(x_0),c(x_0)\}, \max_{u_0}\min_{d_0}\max_{u_1}\min_{d_1}\dots \max_{t=1,\dots,\infty} \min\{ \\& \min\{ \gamma^t r(\xi_{x_0}^{\mathbf{u,d}}(t)),\min_{t'=1,\dots,t}\gamma^{t'} c(\xi_{x_0}^{\mathbf{u,d}}(t')) \},c(x_0) \} \Big\} \\
% = &\max\Big\{ \min\{r(x_0),c(x_0)\},  \min\{ \inf_{\phi}\max_{\{u_t\}_{t=0}^\infty} \sup_{t=1,2,\dots} \\&\min\{\gamma^t r(\xi_{x_0}^{\mathbf{u},\phi(\mathbf{u})}(t)), \min_{\tau=1,\dots,t}\gamma^{\tau} c(\xi_{x_0}^{\mathbf{u},\phi(\mathbf{u})}(\tau))\} , c(x_0)\} \Big\} \\
% = &\max\Big\{ \min\{ r(x_0),c(x_0) \}, \min \big\{\gamma \inf_{\phi}\max_{\{u_t\}_{t=0}^\infty} \sup_{\tilde{t} = 0,1,\dots}\min \{\\&   \gamma^{\tilde{t}} r(\xi_{x_0}^{\mathbf{u},\phi(\mathbf{u})}(\tilde{t}+1)), \min_{\tilde{t}' = 0,\dots, t} \gamma^{\tilde{t}'}c(\xi^{\mathbf{u},\phi(\mathbf{u})}_{x_0}(\tilde{t}'+1)) \}, c(x_0) \big\} \Big\}\\
% =&\max\Big\{ \min\{ r(x_0),c(x_0) \}, \min \big\{\gamma \max_{u_0}\min_{d_0}\inf_{\phi}\max_{\{u_t\}_{t=1}^\infty} \sup_{\tilde{t} = 0,1,\dots}\\&  \min \{ \gamma^{\tilde{t}} r(\xi_{x_0}^{\mathbf{u},\phi(\mathbf{u})}(\tilde{t}+1)), \min_{\tilde{t}' = 0,\dots, t}\\& \gamma^{\tilde{t}'}c(\xi^{\mathbf{u},\phi(\mathbf{u})}_{x_0}(\tilde{t}'+1)) \}, c(x_0) \big\} \Big\} \\
% =& \max\Big\{ \min\{ r(x_0),c(x_0) \}, \min \{c(x_0) ,\\& \gamma \max_{u_0}\min_{d_0} V(f(x_0,u_0,d_0))\} \Big\}\\
\valuepure(x_0)= &\min\Big\{ c(x_0), \max\{ r(x_0) , \gamma \max_{u_0}\min_{d_0} \valuepure(f(x_0,u_0,d_0)) \} \Big\}.
\end{aligned}
\end{equation*}
% where the first equality results from Lemma~\ref{lem: max_min_swap}, the third equality follows from \eqref{eq:max_min_swap_eq} and the last equality follows from the observation that for all $ a,b,c\in\mathbb{R}$,
% $\max\big\{ \min\{a,b\} ,\min\{ b,c \} \big\} = \min \big\{b, \max\{ a,c \} \big\}$.
%Lemma~\ref{lem:double_min}.
%Let $\pi^*$ be the optimal policy. Without loss of generality, at the time $t=0$, we have four cases: (1) $r(s_0)> \gamma \max_{a_0} V(s_1)$ and $c(s_0)\le r(s_0)$; (2) $ r(s_0) > \gamma \max_{a_0} V(s_1) $ and $ c(s_0)> r(s_0) $; (3) $ r(s_0)\le \gamma \max_{a_0} V(s_1) $ and $c(s_0) \le \gamma \max_{a_0} V(s_1) $; (4) $ r(s_0)\le \gamma \max_{a_0} V(s_1) $ and $ c(s_0)> \gamma \max_{a_0} V(s_1)$.
%For the first case, we have 
%\begin{equation}
%    \begin{aligned}
%    r(s_0) &> \gamma \max_{a_0}V(s_1)\\
%    & = \left.\gamma \max_{t=1,\dots,\infty}\min \{ \gamma^t r(s_t), \min_{t'=1,\dots, t} \gamma^{t'}c(s_{t'}) \}\right|_{\pi^*}\\
%    & = 
%    \end{aligned}
%\end{equation}
\noindent Next, we show that \eqref{eq:bellman_backup} is a contraction mapping by proving that %Let $V^{(0)}(\cdot):\mathbb{R}^n\to \mathbb{R}^n$ be an arbitrary bounded function. For each non-negative integer $k$, we define 
%\begin{equation*}
%V^{(k+1)}(x): = \min \{ c(x), \max\{ r(x),\gamma \max_u \min_d V^{(k)}(f(x,u,d)) \} \}. 
%\end{equation*}
for all $x$, $| B[V_1](x) - B[V_2](x) |\le \gamma \left\| V_1 - V_2 \right\|_{\infty}$, where $V_1$ and $V_2$ are two arbitrary bounded functions. One can write \begin{equation}\label{eq:proof_Bellman_backup1}\small
    \begin{aligned}
    &|B[V_1] (x) - B[V_2](x)|\\%& = |\min\{c(x),\max\{r(x),\gamma \max_u\min_d V_k(f(x,u,d))\}\} \\&\ \ -\min\{c(x),\max\{r(x), \gamma \max_u \min_d V_{k-1}(f(x,u,d))\}\}| \\
    &\le | \max\{ r(x), \gamma \max_u\min_d V_1(f(x,u,d)) \}\\&\  \ - \max\{ r(x),\gamma \max_{u}\min_d V_2 (f(x,u,d)) \}|\\
    &\le | \gamma \max_u \min_d V_1(f(x,u,d))  - \gamma \max_u \min_d V_2(f(x,u,d))|
    \end{aligned}
\end{equation}
where the above inequalities follow from the fact that $\|\min\{a,b\} - \min\{a,c\}\|\le b-c, \forall a,b,c\in\mathbb{R}$.
% \begin{equation}
%     \begin{aligned}
%     \|\min\{a,b\} - \min\{a,c\}\|\le b-c, \forall a,b,c\in\mathbb{R}
%     \end{aligned}
% \end{equation}
%Lemma~\ref{lemma:min_max_inequality}.
%Without loss of generality, we 
Suppose $\max_u\min_d V_1(f(x,u,d))\ge \max_u\min_d V_2(f(x,u,d))$ and $u^*:=\argmax_u \min_d V_1(f(x,u,d))$. In addition, let $d^*:=\arg\min_d V_2(f(x,u^*,d))$. We have
\begin{equation}\label{eq:proof_Bellman_backup2}\small
    \begin{aligned}
    |\gamma &\max_u\min_d V_1(f(x,u,d))-\gamma \max_u\min_d V_2 (f(x,u,d))|\\&\le \gamma |\min_d V_1( f(x,u^*,d) ) - \min_d V_2(f(x,u^*,d))|\\
    % & \le \gamma \max_u |\min_d V_k(f(x,u,d)) - \min_d V_{k-1}(f(x,u,d))| \\
    & \le \gamma | V_1(f(x,u^*,d^*)) - V_2(f(x,u^*,d^*)) |\\
    & \le \gamma \max_{x} |V_1(x) - V_2(x)|
    \le \gamma \|V_1 - V_2\|_{\infty}.
    \end{aligned}
\end{equation}
From \eqref{eq:proof_Bellman_backup1} to \eqref{eq:proof_Bellman_backup2}, we have $|B[V_1](x) - B[V_2](x)|\le \gamma \| V_1 - V_2\|_\infty,\ \forall x$, 
%\begin{equation*}
%    \begin{aligned}
%    |B[V_1](x) - B[V_2](x)|\le \gamma \| V_1 - V_2\|_\infty,\ \textrm{for all }x,
%    \end{aligned}
%\end{equation*}
implying $\| B[V_1] - B[V_2] \|_\infty\le \gamma \| V_1 - V_2 \|_\infty$.
\end{proof}

\begin{proof}[Proof of Theorem~\ref{lemma:continuity}]
Define 
\begin{align*}\small
    P(\controlpolicy,\disturbancepolicy,t,x) \coloneqq \min\{ \gamma^t r(\xi_x^{\mathbf{u},\mathbf{d}}(t)), \min_{\tau=0,...,t} \gamma^\tau c(\xi_x^{\mathbf{u},\mathbf{d}}(\tau)) \}.
\end{align*}

Consider two initial states $x_1,x_2\in\mathbb{R}^n$.
Given $\epsilon>0$, there exists a non-anticipative strategy $\bar{\phi}$ such that
\begin{align}\small
    V(x_1) \geq \sup_\mathbf{u} \sup_t P(\mathbf{u},\bar{\phi}(\mathbf{u}), t,x_1) - \epsilon.
    \label{eq:pf_lma_cont_eq1}
\end{align}
We select a control sequence $\bar{\mathbf{u}}$ and time $\bar{t}$ such that $V(x_2) \leq  P(\bar{\mathbf{u}},\bar{\phi}(\bar{\mathbf{u}}), \bar{t},x_2) + \epsilon$. 
% \begin{align}\small
%     V(x_2) \leq  P(\bar{\mathbf{u}},\bar{\phi}(\bar{\mathbf{u}}), \bar{t},x_2) + \epsilon.
%     \label{eq:pf_lma_cont_eq2}
% \end{align}
Moreover, \eqref{eq:pf_lma_cont_eq1} implies that $V(x_1) \geq  P(\bar{\mathbf{u}},\bar{\phi}(\bar{\mathbf{u}}), \bar{t},x_1) - \epsilon$. 
% \begin{align}\small
%     V(x_1) \geq  P(\bar{\mathbf{u}},\bar{\phi}(\bar{\mathbf{u}}), \bar{t},x_1) - \epsilon.
%     \label{eq:pf_lma_cont_eq3}
% \end{align}
%By combining \eqref{eq:pf_lma_cont_eq2} and \eqref{eq:pf_lma_cont_eq3}, we obtain
Combining these inequalities, we have
\begin{equation}\small
\begin{aligned}
    V(x_1)  - V(x_2 ) + &2\epsilon \geq P(\bar{\mathbf{u}},\bar{\phi}(\bar{\mathbf{u}}), \bar{t},x_1) - P(\bar{\mathbf{u}},\bar{\phi}(\bar{\mathbf{u}}), \bar{t},x_2) \\
    % = & \min\{ \gamma^{\bar{t}} r(\xi_{x_1}^{\bar{\mathbf{u}},\bar{\phi}(\bar{\mathbf{u}})}(\bar{t})), \min_{\tau=0,...,\bar{t}} \gamma^\tau c(\xi_{x_1}^{\bar{\mathbf{u}},\bar{\phi}(\bar{\mathbf{u}})}(\bar{t})) \}\\
    % -& \min\{ \gamma^{\bar{t}} r(\xi_{x_2}^{\bar{\mathbf{u}},\bar{\phi}(\bar{\mathbf{u}})}(\bar{t})), \min_{\tau=0,...,\bar{t}} \gamma^\tau c(\xi_{x_2}^{\bar{\mathbf{u}},\bar{\phi}(\bar{\mathbf{u}})}(\bar{t})) \}\\
    \geq & \min\{ \gamma^{\bar{t}} (r(\xi_{x_1}^{\bar{\mathbf{u}},\bar{\phi}(\bar{\mathbf{u}})}(\bar{t}))-r(\xi_{x_2}^{\bar{\mathbf{u}},\bar{\phi}(\bar{\mathbf{u}})}(\bar{t}))),\\
    &\min_{\tau=0,...,\bar{t}} \gamma^\tau (c(\xi_{x_1}^{\bar{\mathbf{u}},\bar{\phi}(\bar{\mathbf{u}})}(\bar{t})) - c(\xi_{x_2}^{\bar{\mathbf{u}},\bar{\phi}(\bar{\mathbf{u}})}(\bar{t}))) \}.
\end{aligned}
\label{eq:pf_lma_cont_eq4}
\end{equation}
The last inequality is due to the fact that for any finite values $a_i,b_i\in \mathbb{R}$ ($i=1,...,n$), we have
\begin{align*}\small
\begin{split}
    \min\{a_1,...,a_n\}&-\min\{b_1,...,b_n\} \geq \min\{a_1-b_1,...,a_n-b_n\}.
\end{split}
\label{eq:pf_lma_cont_eq5}
\end{align*}
According to the Lipscthiz-continuity assumptions, 
\begin{align}\small
\begin{split}
    & \|\xi_{x_1}^{\mathbf{u},\mathbf{d}}(t) - \xi_{x_2}^{\mathbf{u},\mathbf{d}}(t)  \| \leq L_f^t\|x_1-x_2\|, \\
    & \|c(\xi_{x_1}^{\mathbf{u},\mathbf{d}}(t)) - c(\xi_{x_2}^{\mathbf{u},\mathbf{d}}(t))  \| \leq L_c L_f^t\|x_1-x_2\|, \\
    & \|r(\xi_{x_1}^{\mathbf{u},\mathbf{d}}(t)) - r(\xi_{x_2}^{\mathbf{u},\mathbf{d}}(t))  \| \leq L_r L_f^t\|x_1-x_2\|.
\end{split}
\end{align}
Thus, it follows from \eqref{eq:pf_lma_cont_eq4} that
\begin{align}\small
\begin{split}
    V&(x_1)  - V(x_2 ) + 2\epsilon  \\
    &\geq-\max\{ L_r \gamma^{\bar{t}}L_f^{\bar{t}}, \max_{\tau=0,...,\bar{t}} L_c \gamma^{\tau}L_f^{\tau } \} \|x_1-x_2\|.
\end{split}
\label{eq:pf_lma_cont_eq55}
\end{align}
The condition $\gamma L_f <1$ implies that the coefficient in the right-hand side in \eqref{eq:pf_lma_cont_eq55} is bounded for all $\bar{t}$. As a result, $   V(x_1)  - V(x_2 ) + 2\epsilon \geq -C \|x_1-x_2\|
$
for some $C>0$. Similarly, we can show that $
%\begin{align}\small
    V(x_2)  - V(x_1 ) + 2\epsilon \geq -C \|x_1-x_2\|.
%    \label{eq:pf_lma_cont_eq7}
%\end{align}
$
Combining these two inequalities, we prove Theorem \ref{lemma:continuity}.
\end{proof}

\begin{lemma}\label{lem:inequality_minimax}
Consider two functions $g(\cdot):\mathbb{R}\to\mathbb{R}$ and $\bar{g}(\cdot):\mathbb{R}\to\mathbb{R}$. Suppose that $g(a,b)\le \bar{g}(a,b)$, $\forall a,b$. Then, we have $\max_a\min_b g(a,b) \le \max_a \min_b \bar{g}(a,b)$.
\end{lemma}
\begin{proof}[Proof of Theorem~\ref{thm:reaching time}]
    By the definition of $\discountedreachavoidmeasure$, we have
    \begin{equation*}
    \begin{aligned}
        &g_{\check{\gamma}}(\xi_x^{\pione, \disturbancepolicy}, \ttwo) \le \check{\gamma}^{\tone} \cdot \check{\gamma}\cdot r_{\textrm{max}} \le \check{\gamma}^{\tone} V_\gamma(x) < \Big(\frac{\check{\gamma}}{\gamma}\Big)^{\tone} V_\gamma(x) \\& \le \Big(\frac{\check{\gamma}}{\gamma}\Big)^{\tone} g_{\gamma}(\xi_x^{\pione, \disturbancepolicy}, \tone)
        % & \le \Big(\frac{\check{\gamma}}{\gamma}\Big)^{\tone} \min\{\gamma^{\tone}r(\xi_x^{\uone, \nonanticipativestrategy(\uone)}(\tone)), \min_{\tau=0,\dots,\tone} \{\gamma^\tau c(\xi_x^{\uone, \nonanticipativestrategy(\uone)}( \tau)\}\} \\
         \le  g_{\check{\gamma}}(\xi_x^{\pione, \disturbancepolicy}, \tone) 
    \end{aligned}
    \end{equation*}
    This completes the proof.
    % \begin{equation}
    %     \Big(\frac{\check{\gamma}}{\gamma}\Big)^t <\Big(\frac{\check{\gamma}}{\gamma}\Big)^{t-1} 
    % \end{equation}
\end{proof}
