# Supplementary material for: Certifiable Reachability Learning Using a New Lipschitz Continuous Value Function
Source: arXiv:2408.07866 source file (2025-02-16)
Supplement: Supplementary file 2 [file new_appendix.tex]

\section{Appendix}
\begin{proof}[Proof of Theorem~\ref{thm:reaching time}]
    By the definition of $\discountedreachavoidmeasure$, we have\vspace{-0.5em}
    \begin{equation*}
    \begin{aligned}
        &g_{\check{\gamma}}(\xi_x^{\pione, \disturbancepolicy}, \ttwo) \le \check{\gamma}^{\tone} \check{\gamma} \max_x r(x) \le \check{\gamma}^{\tone} V_\gamma(x) < \big(\check{\gamma}/\gamma\big)^{\tone} V_\gamma(x) \\& \le \big(\check{\gamma}/\gamma\big)^{\tone} g_{\gamma}(\xi_x^{\pione, \disturbancepolicy}, \tone)
        % & \le \Big(\frac{\check{\gamma}}{\gamma}\Big)^{\tone} \min\{\gamma^{\tone}r(\xi_x^{\uone, \nonanticipativestrategy(\uone)}(\tone)), \min_{\tau=0,\dots,\tone} \{\gamma^\tau c(\xi_x^{\uone, \nonanticipativestrategy(\uone)}( \tau)\}\} \\
         \le  g_{\check{\gamma}}(\xi_x^{\pione, \disturbancepolicy}, \tone) \qed
    \end{aligned}
    \end{equation*}
    % This completes the proof.
    % \begin{equation}
    %     \Big(\frac{\check{\gamma}}{\gamma}\Big)^t <\Big(\frac{\check{\gamma}}{\gamma}\Big)^{t-1} 
    % \end{equation}
% \vspace{-1em}
\end{proof}\vspace{-1em}
